# Supplementary material for: Interpretable Memory Models for Spaced Repetition
Source: arXiv:2610.10548 source file (2026-09-14)
Supplement: Supplementary file 1 [file 9_appendix.tex]

\begin{table}[H]
\centering
\small
\begin{tabular*}{\columnwidth}{l@{\extracolsep{\fill}}rrrr}
\toprule
& \multicolumn{2}{c}{\textbf{SBD}} & \multicolumn{2}{c}{\textbf{SBD binary}} \\
\cmidrule(lr){2-3} \cmidrule(lr){4-5}
\textbf{Weight} & \textbf{Value} & \textbf{$\sigma$} & \textbf{Value} & \textbf{$\sigma$} \\
\midrule
$w_{1}$ & 1.7392 & 0.5003 & 2.1210 & 0.5003 \\
$w_{2}$$^{\dagger}$ & 0.1122 & 0.5460 & 0.1721 & 0.5460 \\
$w_{3}$ & 0.5298 & 0.0989 & 0.4579 & 0.0989 \\
\addlinespace
$w_{4}$$^{\dagger}$ & 0.3610 & 1.3437 & 0.3157 & 1.1018 \\
$w_{5}$$^{\dagger}$ & 4.0417 & 0.4113 & 2.4905 & 0.4113 \\
\addlinespace
$w_{6}$$^{\dagger}$ & 0.0606 & 1.7540 & 0.1583 & 1.7540 \\
$w_{7}$$^{\dagger}$ & 0.4963 & 0.7778 & 0.6506 & 0.7778 \\
\bottomrule
\end{tabular*}
\caption{Pretraining weights for SBD and its binary version, with the prior
width $\sigma$ used for fine-tuning. Weights marked $\dagger$ are regularized in log space. The prior is placed
on the fitted parameters, and $\sigma$ for $w_2$, $w_4$, and $w_5$ is the
implied width with the other weights held fixed.}
\label{weights-table}
\end{table}
